# Supplementary material for: Planning to Practice: Efficient Online Fine-Tuning by Composing Goals in Latent Space
Source: arXiv:2205.08129 source file (2023-04-18)
Supplement: Supplementary file 1 [file 7-appendix.tex]

\subsection{Simulation Experimental Details}
\label{appendix:simulation_experimental_details}
Our simulated dataset consists of 4,000 trajectories (300,000 transitions). Every 4 trajectories, we randomize the position and orientation of the drawer, slidable object, and graspable object in the following ways. The position of the drawer is randomly selected between the back two quadrants. The orientation of the drawer is randomly selected such that it doesn't collide into the surrounding wall. The position of the slidable object is randomly selected between the four quadrants such that it doesn't collide with the drawer. The position of the graspable object is randomly selected between inside the drawer, on top of the drawer, or on top of the table. If the graspable object is on top of the table, its position on top of the table is randomly selected such that it doesn't collide with the drawer or slidable object. The yaw of the graspable object is randomized. 
